# Supplementary material for: Towards Valid and Reliable Privacy Concern Scales: The Example of IUIPC-8
Source: arXiv:2308.08322 source file (2023-08-16)
Supplement: Supplementary file 1 [file IUIPC-8_FA_Supplementary-concordance.tex]

\Sconcordance{concordance:IUIPC-8_FA_Supplementary.tex:IUIPC-8_FA_Supplementary.Rnw:%
1 4 1 50 0 1 5 81 1 1 4 2 1 16 %
0 2 1 1080 0 103 1}
